# Supplementary material for: Spatio-Temporal Patterns of the International Merger and Acquisition Network
Source: arXiv:1703.04899 source file (2017-07-13)
Supplement: Supplementary file 1 [file SI.pdf]

# Spatio-Temporal Patterns of the International Merger and Acquisition Network

## Supplementary Information

**Marco Dueñas<sup>1,\*</sup>, Rossana Mastrandrea<sup>2</sup>, Matteo Barigozzi<sup>3</sup>, and Giorgio Fagiolo<sup>4</sup>**

<sup>1</sup>Department of Economics, International Trade and Social Policy, Universidad de Bogotá Jorge Tadeo Lozano, Bogotá

<sup>2</sup>IMT School for Advanced Studies, Lucca

<sup>3</sup>Department of Statistics, London School of Economics and Political Science, London

<sup>4</sup>Istituto di Economia, Scuola Superiore Sant'Anna, Pisa

\*E-mail: marcoa.duenase@utadeo.edu.co (corresponding author)

### Country Groups

#### Group 1

Argentina; Australia; Belgium; Bermuda; Brazil; British Virgin; Canada; Chile; China; Denmark; Finland; France; Germany; Hong Kong; India; Ireland-Rep; Israel; Italy; Japan; Luxembourg; Malaysia; Mexico; Netherlands; New Zealand; Norway; Philippines; Portugal; Singapore; South Africa; South Korea; Spain; Sweden; Switzerland; Taiwan; Thailand; United Kingdom; United States.

#### Group 2

Antigua and Barbuda; Armenia; Austria; Azerbaijan; Bahamas; Bahrain; Bangladesh; Barbados; Belize; Bolivia; Bosnia and Herzegovina; Botswana; Brunei; Bulgaria; Cambodia; Cayman Islands; Colombia; Congo; Costa Rica; Croatia; Cuba; Cyprus; Czech Republic; Dominican Rep; Ecuador; Egypt; El Salvador; Estonia; Fiji; Ghana; Gibraltar; Greece; Guam; Guatemala; Guernsey; Hungary; Iceland; Indonesia; Iraq; Isle of Man; Ivory Coast; Jamaica; Jersey; Jordan; Kazakhstan; Kenya; Kuwait; Latvia; Lebanon; Libya; Liechtenstein; Lithuania; Macao; Macedonia; Malta; Mauritius; Monaco; Mongolia; Montenegro; Morocco; New Caledonia; Nigeria; Oman; Pakistan; Panama; Papua New Guinea; Peru; Poland; Puerto Rico; Qatar; Romania; Russian Federation; Saudi Arabia; Serbia; Seychelles; Slovak Rep; Slovenia; Sri Lanka; Sudan; Trinidad & Tobago; Tunisia; Turkey; Turks/Caicos; Ukraine; United Arab Emirates; Uruguay; US Virgin Is; Uzbekistan; Venezuela; Vietnam; Western Samoa; Zambia; Zimbabwe.

#### Group 3

Afghanistan; Albania; Algeria; American Samoa; Andorra; Angola; Anguilla; Aruba; Belarus; Benin; Bhutan; Burkina Faso; Burundi; Cameroon; Cape Verde; Central African Republic; Chad; Comoros; Cook Islands; Democratic Republic of Congo; Djibouti; Dominica; Equatorial Guinea; Eritrea; Ethiopia; Falkland Islands; Faroe Islands; French Polynesia; Gabon; Gambia; Georgia; Greenland; Grenada; Guadeloupe; Guinea; Guinea-Bissau; Guyana; Haiti; Honduras; Iran; Kiribati; Kyrgyzstan; Laos; Lesotho; Liberia; Madagascar; Malawi; Maldives; Mali; Marshall Islands; Martinique; Mauritania; Mayotte; Micronesia; Moldova; Mozambique; Myanmar(Burma); N. Mariana; Namibia'; Nauru; Nepal; Nicaragua; Niger; Niue; Norfolk Island; North Korea; Palau; Palestine; Paraguay; Reunion; Rwanda; Saint Vincent and the Grenadines; San Marino; Sao Tome; Senegal; Sierra Leone; Solomon Islands; Somalia; St Kitts & Nevis; St Lucia; Suriname; Swaziland; Syria; Tajikistan; Tanzania; Timor-Leste; Togo; Tokelau; Tonga; Turkmenistan; Tuvalu; Uganda; Vanuatu; Yemen.

### Network Topology

We test whether the empirical probability distribution of node out-degree differ from that of node in-degree (we call this set of tests “between” tests). Furthermore, we test whether in-degree probability distributions differ across the years (we call this set of tests “within” tests), and similarly for out-degree probability distributions. Table 1 shows two-sample Kolmogorov-Smirnov (K-S) tests within and between the distributions of  $ND_{in}$  and  $ND_{out}$  in different years. In the case of the distribution of  $ND_{in}$ , the null hypothesis of K-S test is almost always rejected, allowing us to conclude that in-degree profiles are quite unstable. Conversely, in the case of the distribution of  $ND_{out}$ , the null hypothesis of the K-S test is most frequently non rejected. This is an expected result because the IMAN is very target oriented and suggests that out-degree profiles are quite similar in different

periods. Finally, the null hypothesis of the K-S test to compare the in-degree and out-degree distributions is always rejected. This highlights that out- and in-degree profiles are very different.

**Table 1.** Two-sample Kolmogorov-Smirnov Tests within and between in- and out-degree distributions in different years.

| Column<br>Year | Within test of In-degree |                   |                |                | Within test of Out-degree |                   |                 |                   | Between test of In-degree vs. Out-degree |                |                |                |                |
|----------------|--------------------------|-------------------|----------------|----------------|---------------------------|-------------------|-----------------|-------------------|------------------------------------------|----------------|----------------|----------------|----------------|
|                | (1)<br>2000              | (2)<br>2003       | (3)<br>2007    | (4)<br>2010    | (5)<br>2000               | (6)<br>2003       | (7)<br>2007     | (8)<br>2010       | (9)<br>1995                              | (10)<br>2000   | (11)<br>2003   | (12)<br>2007   | (13)<br>2010   |
| 1995           | 0.12<br>(0.35)           | 0.05***<br>(1.00) | 0.12<br>(0.30) | 0.11<br>(0.42) | 0.07*<br>(0.92)           | 0.06**<br>(0.98)  | 0.13<br>(0.25)  | 0.10<br>(0.60)    | 0.31<br>(0.00)                           | 0.24<br>(0.00) | 0.25<br>(0.00) | 0.30<br>(0.00) | 0.27<br>(0.00) |
| 2000           |                          | 0.10<br>(0.53)    | 0.08<br>(0.70) | 0.07<br>(0.89) |                           | 0.05***<br>(1.00) | 0.07*<br>(0.91) | 0.05***<br>(0.99) |                                          | 0.23<br>(0.00) | 0.24<br>(0.00) | 0.29<br>(0.00) | 0.26<br>(0.00) |
| 2003           |                          |                   | 0.09<br>(0.62) | 0.09<br>(0.64) |                           |                   | 0.08<br>(0.79)  | 0.06*<br>(0.92)   |                                          |                | 0.21<br>(0.00) | 0.26<br>(0.00) | 0.23<br>(0.00) |
| 2007           |                          |                   |                | 0.07<br>(0.85) |                           |                   |                 | 0.04***<br>(1.00) |                                          |                |                | 0.32<br>(0.00) | 0.30<br>(0.00) |
| 2010           |                          |                   |                |                |                           |                   |                 |                   |                                          |                |                |                | 0.32<br>(0.00) |

*Notes:* The null hypotheses tested in columns (1-4) and (5-8) are that the observed distributions come from the same distributions, within in-degree and out-degree distributions, respectively. The null hypotheses tested in columns (9-13) are that the observed distributions between in-degree and out-degree come from the same distributions. The p-values are reported in parenthesis. Significance level: \*\*\* p<0.01, \*\* p<0.05, \* p<0.10.

Table 2 presents the top-10 ranking of countries with high node degree (*ND*) and node strength (*NS*). Here, we are interested in the co-occurrence of rankings of total country's M&As (i.e., node-strength) and the country's number of partners (i.e., node degree), distinguishing among in- and out-oriented statistics. Comparing within statistics across different years, for both *ND* and *NS*, we observe high co-occurrence of several high-income economies. Although the order in which they appear changes from year to year, some countries, such as the USA and GBR, appear recurrently in the top of the rankings. Interestingly, we observe in the rankings a few emergent economies, as China, which appears in 2000 as the target of high-volume inflows and in 2010 as an acquirer with very high outflows.

**Table 2.** Node degree and node strength rankings.

| 1995        |     | 2000 |     | 2003 |     | 2007 |     | 2010 |     |
|-------------|-----|------|-----|------|-----|------|-----|------|-----|
| Node Degree |     |      |     |      |     |      |     |      |     |
| in          | out | in   | out | in   | out | in   | out | in   | out |
| USA         | USA | USA  | USA | USA  | USA | USA  | GBR | GBR  | USA |
| GBR         | GBR | GBR  | GBR | GBR  | GBR | GBR  | USA | USA  | GBR |
| DEU         | CAN | CAN  | FRA | DEU  | CAN | CAN  | AUS | AUS  | CAN |
| FRA         | DEU | BRA  | DEU | AUS  | NLD | DEU  | CAN | CAN  | AUS |
| AUS         | NLD | AUS  | NLD | FRA  | DEU | AUS  | NLD | FRA  | NLD |
| HKG         | FRA | FRA  | ITA | CHI  | FRA | CHI  | FRA | DEU  | DEU |
| CAN         | JPN | HKG  | CAN | IND  | CHE | IND  | ESP | NLD  | SGP |
| ITA         | SGP | NLD  | SWE | NLD  | ESP | NLD  | RUS | ITA  | SWE |
| NLD         | AUS | DEU  | BEL | HKG  | JPN | RUS  | DEU | CHI  | HKG |
| ESP         | CHE | JPN  | JPN | CHE  | HKG | FRA  | JPN | IND  | IND |

| Node-Strength |     |     |     |     |     |     |     |     |     |
|---------------|-----|-----|-----|-----|-----|-----|-----|-----|-----|
| in            | out | in  | out | in  | out | in  | out | in  | out |
| USA           | USA | USA | GBR | USA | USA | USA | USA | USA | USA |
| GBR           | GBR | DEU | FRA | GBR | GBR | GBR | GBR | GBR | GBR |
| AUS           | DEU | GBR | USA | DEU | DEU | CAN | FRA | BRA | CAN |
| CAN           | CAN | CAN | DEU | FRA | CAN | DEU | DEU | DEU | CHI |
| SWE           | FRA | CHI | ESP | CHE | AUS | NLD | CAN | CAN | JPN |
| FRA           | CHE | FRA | HKG | ITA | NLD | FRA | ITA | AUS | IND |
| DEU           | NLD | NLD | CHE | JPN | FRA | ESP | NLD | FRA | NLD |
| ITA           | SWE | BRA | NLD | NLD | CHE | AUS | ESP | NLD | DEU |
| CHE           | ITA | ESP | CAN | AUS | JPN | ITA | AUS | CHI | FRA |
| NLD           | BEL | SWE | SWE | ESP | MEX | CHE | SWE | ESP | ESP |

The rankings suggest that there exists a positive relation between the number of targets and the outflow volumes, and, similarly, between the number of acquiring countries and the inflow volumes. Figure 1a and Figure 1b show the scatter plots between node degree and node strength.

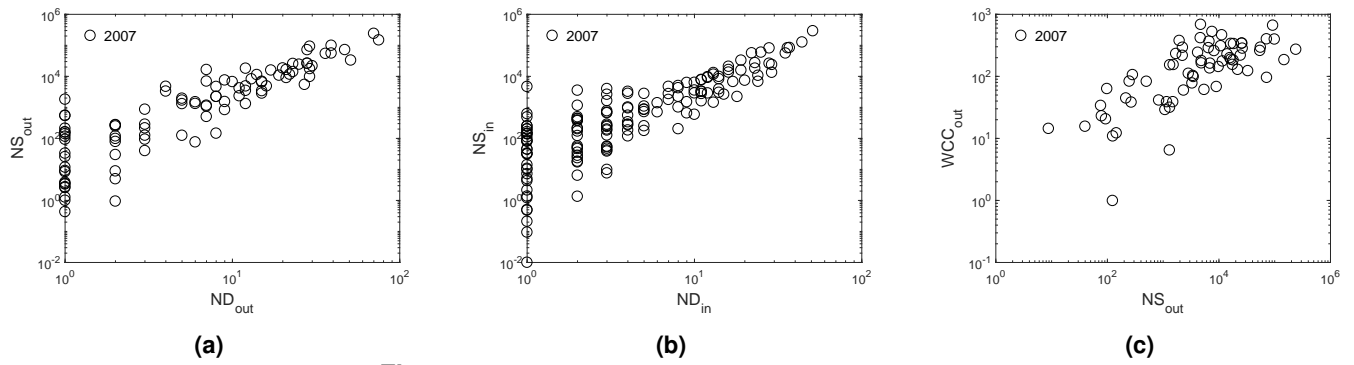

**Figure 1. Scatter plots of network statistics in 2017.**

**Table 3. Binary and weighted clustering coefficient rankings.**

| 1995                     | 2000                | 2003                 | 2007           | 2010             |
|--------------------------|---------------------|----------------------|----------------|------------------|
| <i>BCC<sub>out</sub></i> |                     |                      |                |                  |
| Cuba                     | Puerto Rico         | Costa Rica           | Dominican Rep. | Puerto Rico      |
| Barbados                 | Dominican Rep.      | Guernsey             | Costa Rica     | Barbados         |
| British Virgin           | Guatemala           | Luxembourg           | Guyana         | Costa Rica       |
| Ireland Rep.             | Bolivia             | Greece               | Bolivia        | Jersey           |
| Luxembourg               | Isle of Man         | Estonia              | Isle of Man    | Isle of Man      |
| <i>BCC<sub>in</sub></i>  |                     |                      |                |                  |
| Kuwait                   | Isle of Man         | Bahamas              | Liechtenstein  | Macao            |
| Indonesia                | Iceland             | Guernsey             | Oman           | Philippines      |
| Luxembourg               | Bahrain             | Jersey               | Vietnam        | Indonesia        |
| Denmark                  | Papua New Guinea    | Netherlands Antilles | Western Samoa  | Qatar            |
| Israel                   | China               | Monaco               | Jersey         | New Zealand      |
| <i>BCC<sub>cyc</sub></i> |                     |                      |                |                  |
| Cuba                     | Puerto Rico         | Trinidad & Tobago    | Bahamas        | US Virgin Is.    |
| Uruguay                  | Antigua and Barbuda | Costa Rica           | Barbados       | Uruguay          |
| British Virgin           | Panama              | Peru                 | Costa Rica     | Liechtenstein    |
| Netherlands Antilles     | Venezuela           | Guernsey             | Gibraltar      | Kazakhstan       |
| Luxembourg               | Guernsey            | Monaco               | Botswana       | Macao            |
| <i>BCC<sub>mid</sub></i> |                     |                      |                |                  |
| Bahamas                  | Puerto Rico         | Trinidad & Tobago    | Bahamas        | Liechtenstein    |
| Netherlands Antilles     | Antigua and Barbuda | Costa Rica           | El Salvador    | Seychelles       |
| Ghana                    | Panama              | Uruguay              | Costa Rica     | Kazakhstan       |
| Luxembourg               | Guernsey            | Guernsey             | Montenegro     | Macao            |
| Denmark                  | Isle of Man         | Jersey               | Botswana       | Bangladesh       |
| <i>WCC<sub>out</sub></i> |                     |                      |                |                  |
| Czechoslovakia**         | Germany             | Luxembourg           | Belarus        | Papua New Guinea |
| Ireland Rep.             | Luxembourg          | Italy                | Qatar          | Puerto Rico      |
| Sweden                   | Spain               | Greece               | El Salvador    | Mexico           |
| Australia                | Belgium             | Israel               | Puerto Rico    | Brazil           |
| Brazil                   | Netherlands         | Portugal             | Hungary        | Bermuda          |
| <i>WCC<sub>in</sub></i>  |                     |                      |                |                  |
| South Africa             | Papua New Guinea    | Ireland-Rep          | Argentina      | Qatar            |
| Italy                    | France              | Israel               | Germany        | New Zealand      |
| Saudi Arabia             | Iceland             | Netherlands Antilles | Iceland        | Bermuda          |
| France                   | Bermuda             | Monaco               | Norway         | Ireland Rep.     |
| Sweden                   | Switzerland         | Guernsey             | New Zealand    | Israel           |
| <i>WCC<sub>cyc</sub></i> |                     |                      |                |                  |
| Netherlands Antilles     | Germany             | Trinidad & Tobago    | Bahamas        | Bermuda          |
| Argentina                | France              | Israel               | Iceland        | Kazakhstan       |
| Sweden                   | Luxembourg          | Monaco               | Germany        | Brazil           |
| Switzerland              | Switzerland         | Luxembourg           | Italy          | Ireland Rep.     |
| Italy                    | Bermuda             | Italy                | France         | Mexico           |
| <i>WCC<sub>mid</sub></i> |                     |                      |                |                  |
| Netherlands Antilles     | Germany             | Trinidad & Tobago    | Iceland        | Kazakhstan       |
| Sweden                   | France              | Luxembourg           | Bahamas        | Bermuda          |
| Switzerland              | Guernsey            | Israel               | Germany        | Mexico           |
| France                   | Spain               | Italy                | El Salvador    | Brazil           |
| Italy                    | Luxembourg          | Ireland Rep.         | France         | United States    |

\*\* Although Czechoslovakia split into two sovereign states in 1993, still in 1995 several firms appear in the database as based in Czechoslovakia.

In contrast, we observe that clustering patterns are more heterogeneous. There are neither well established nor persistent hubs in the network. Table 3 shows the top-5 positions for all directed clustering types. The heterogeneity along time and between clustering types is the reason behind the weak and fluctuating correlations among clustering and node degree and node strengths. Figure 1c shows the scatter plot between node strength and clustering correlation.

## Spatial Analysis

The left panel of Figure 2a shows the kernel-density estimation of the distribution of the entries of the geographical-distance matrix (in logs) in 2007. The estimated distribution is left-skewed and bimodal with a higher peak at farther distances. These patterns are robust over time. The Q-Q plots in Figure 2b compare the distributions for different years. We observe a linear relation among the quantiles of the distributions, which suggests that the shapes of the distributions are quite stable.

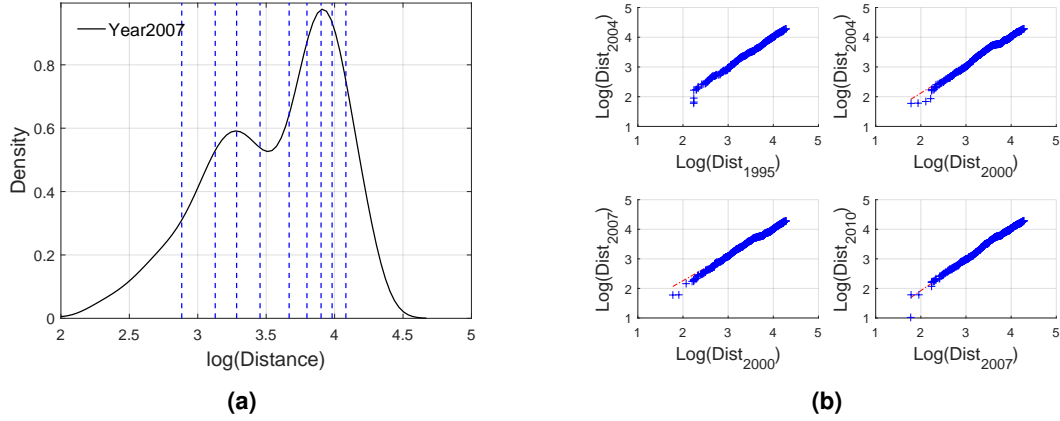

**Figure 2. The distribution of geographical distance between country pairs with M&As. (a)** Kernel estimation for 2007, vertical lines indicate the deciles of the distribution. **(b)** Q-Q plots comparing distributions of different years.
